# Supplementary material for: DISCO: DISCovering Overfittings as Causal Rules for Text Classification Models
Source: arXiv:2411.04649 source file (2024-11-07)
Supplement: Supplementary file 1 [file a.appendix.tex]

\appendix

% \appendix
\section{Appendix of RQ1} 
% \subsection{Appendix: RQ1} 

\section{RQ2-Decoys}
To evaluate the interpretability of our approach on \bert, we utilized adversarial text decoys, which have been employed in prior research\cite{bertdecoy2022wang}.
In the context of RQ2, we provide a comprehensive list of the decoys utilized, as shown in Table~\ref{tab:rq2-decoys}.

\section{Counterfactual Examples}
\label{app:rq1-counterfactual}
Table~\ref{tab:counterfactual} provides a glimpse of selected counterfactual examples.
Notably, certain rules, such as \textit{don't even} $\longrightarrow$ \textbf{NEG} for \movies~and \textit{in its} $\longrightarrow$ \textbf{POS} for \sst, indicate that the model has learned shortcuts between sequences and labels.
When the model acquires incorrect associations, it is prone to making predictions solely based on these misleading sequences, disregarding their contextual significance.
This observation aligns with the behavior exhibited by the model during the causality check for the generated counterfactuals.
Although these counterfactuals share the same predictions as their corresponding rules, the context either lacks label bias (\sst) or demonstrates a bias towards the opposing label (\movies, \multirc).

Furthermore, Table~\ref{tab:counterfactual} presents instances of rules identified by human assessors as ``wrong reasons'' for predictive tasks in RQ3.
Notably, phrases such as ``\underline{of the world trade center}'' or ``\underline{but the algarve}'' are irrelevant to the classification task but are nonetheless exploited as shortcuts by the models.
This indicates that such shortcut patterns detrimentally impact downstream generalization capabilities.
